# Supplementary material for: Lift3D: Synthesize 3D Training Data by Lifting 2D GAN to 3D Generative Radiance Field
Source: arXiv:2304.03526 source file (2023-04-07)
Supplement: Supplementary file 1 [file 12_appendix.tex]

\appendix
\label{sec:appendix}

\twocolumn[{%
\renewcommand\twocolumn[1][]{#1}%
\begin{center}
    {\bf \Large Lift3D: Synthesize 3D Training Data\protect\\ by Lifting 2D GAN to 3D Generative Radiance Field\\[4pt]
    Supplementary Material}
\end{center}
}]

The supplementary material is organized as follows. Sec.~\ref{sec:interp} describes the detailed configurations used in StyleGAN2 interpretation. Sec.~\ref{sec:con_nerf} provides the network structure of NeRF used in Lift3D. Sec.~\ref{sec:sam_p} introduces the sampling parameters used in composition. Sec.~\ref{sec:mvc} verifies the multi-view consistency of our 3D generation framework.

\section{Interpretation of StyleGAN2}\label{sec:interp}

% After derived disentanglement information from GANSpace~\cite{ganspace} that the first eight layers of latents roughly control the pose of objects, our goal is to ``annotate'' pose label of corresponding latents. We first use Blender EEVEE engine~\cite{blender2018blender} to render a ShapeNet~\cite{chang2015shapenet} model under 200 different views $\mathbf{P}$, ranging from $0-360^{\circ}$ in azimuth, and $0-20^{\circ}$ in elevation. The rendered images thus naturally contain accurate ground truth pose labels. 

We derive disentanglement of latent space in StyleGAN2~\cite{Karras2020stylegan2} from GANSpace~\cite{ganspace}. We disentangle StyleGAN2 and identify the first eight layers latents as the latents that control the object pose and the other eight layers latents as the latents that control the attributes except object shape.  In Lift3D, our goal is to annotate these latents with pose labels for lifting process. We first use Blender EEVEE engine~\cite{blender2018blender} to render a ShapeNet~\cite{chang2015shapenet} model under 200 different views $\mathbf{P}$, ranging from $0-360^{\circ}$ in azimuth, and $0-20^{\circ}$ in elevation. The rendered images thus naturally contain accurate ground truth pose labels. 

With a fixed pretrained StyleGAN2~\cite{Karras2020stylegan2}, we initialize 200 different latents $\mathbf{z} \in \mathbb{R}^{512}$ from Gaussian distribution $\mathbf{Z}\in\mathcal{N}(0, \mathbf{I})$. The latents $\mathbf{z}$ are mapped to $\mathbf{w} \in  \!\mathbb{R}^{16\times 512}$ by the mapping network in StyleGAN2. We optimize the latents $\mathbf{w}$ using Adam~\cite{kingma2014adam} optimizer with learning rate of 1e-3 for 5000 iterations. The loss function is a simple $L1$ loss. After optimization, the first eight layers of latents $\mathbf{w}$ are annotated with ``pseudo'' pose labels, as the disentanglement and interpretation process is non-perfect.

% We follow EG3D~\cite{Chan2022} to build our conditional NeRF.

\section{Conditional NeRF}\label{sec:con_nerf}

Our conditional NeRF mainly builds upon EG3D~\cite{Chan2022}. Fig.~\ref{fig:nerf_supp} depicts the detailed structure of NeRF in Lift3D. The overall network composes two parts: the mapping network and the synthesis network. The mapping network contains 8-layer MLPs and 16 affine transformations that maps the randomly sampled noise latents $z\in  \!\mathbb{R}^{512}$ to $w\in  \!\mathbb{R}^{16\times 512}$. The latents are then modulate the synthesis network to generate orthogonal tri-planes that form the axis-aligned feature grid. The feature planes are of size $N \times N \times (C \times 3)$, where $N = 256$ denotes the spatial resolution and $C = 32$ the feature dimension. Any sampled 3D point $x\in  \!\mathbb{R}^{3}$ of volumetirc rendering is projected onto the three feature planes to retrieve its interpolated feature vector. The final SIREN-based~\cite{sitzmann2020siren} MLP that condition on the mean of $w$ then convert the feature vector to the RGB and density value.

% , we query its feature vector by projecting it onto each of the three feature planes, retrieving the corresponding three feature vectors via bilinear interpolation, then summing the three as the final feature vector. To further incorporate global information, we then feed the final feature vector to a single layer SIREN-based~\cite{sitzmann2020siren} MLP that conditions on $\mathbf{{z}}$ to output the density and RGB value.

\begin{figure}[t!]
    \centering
    \includegraphics[width = 0.48\textwidth, trim = 0 0 0 0, clip]{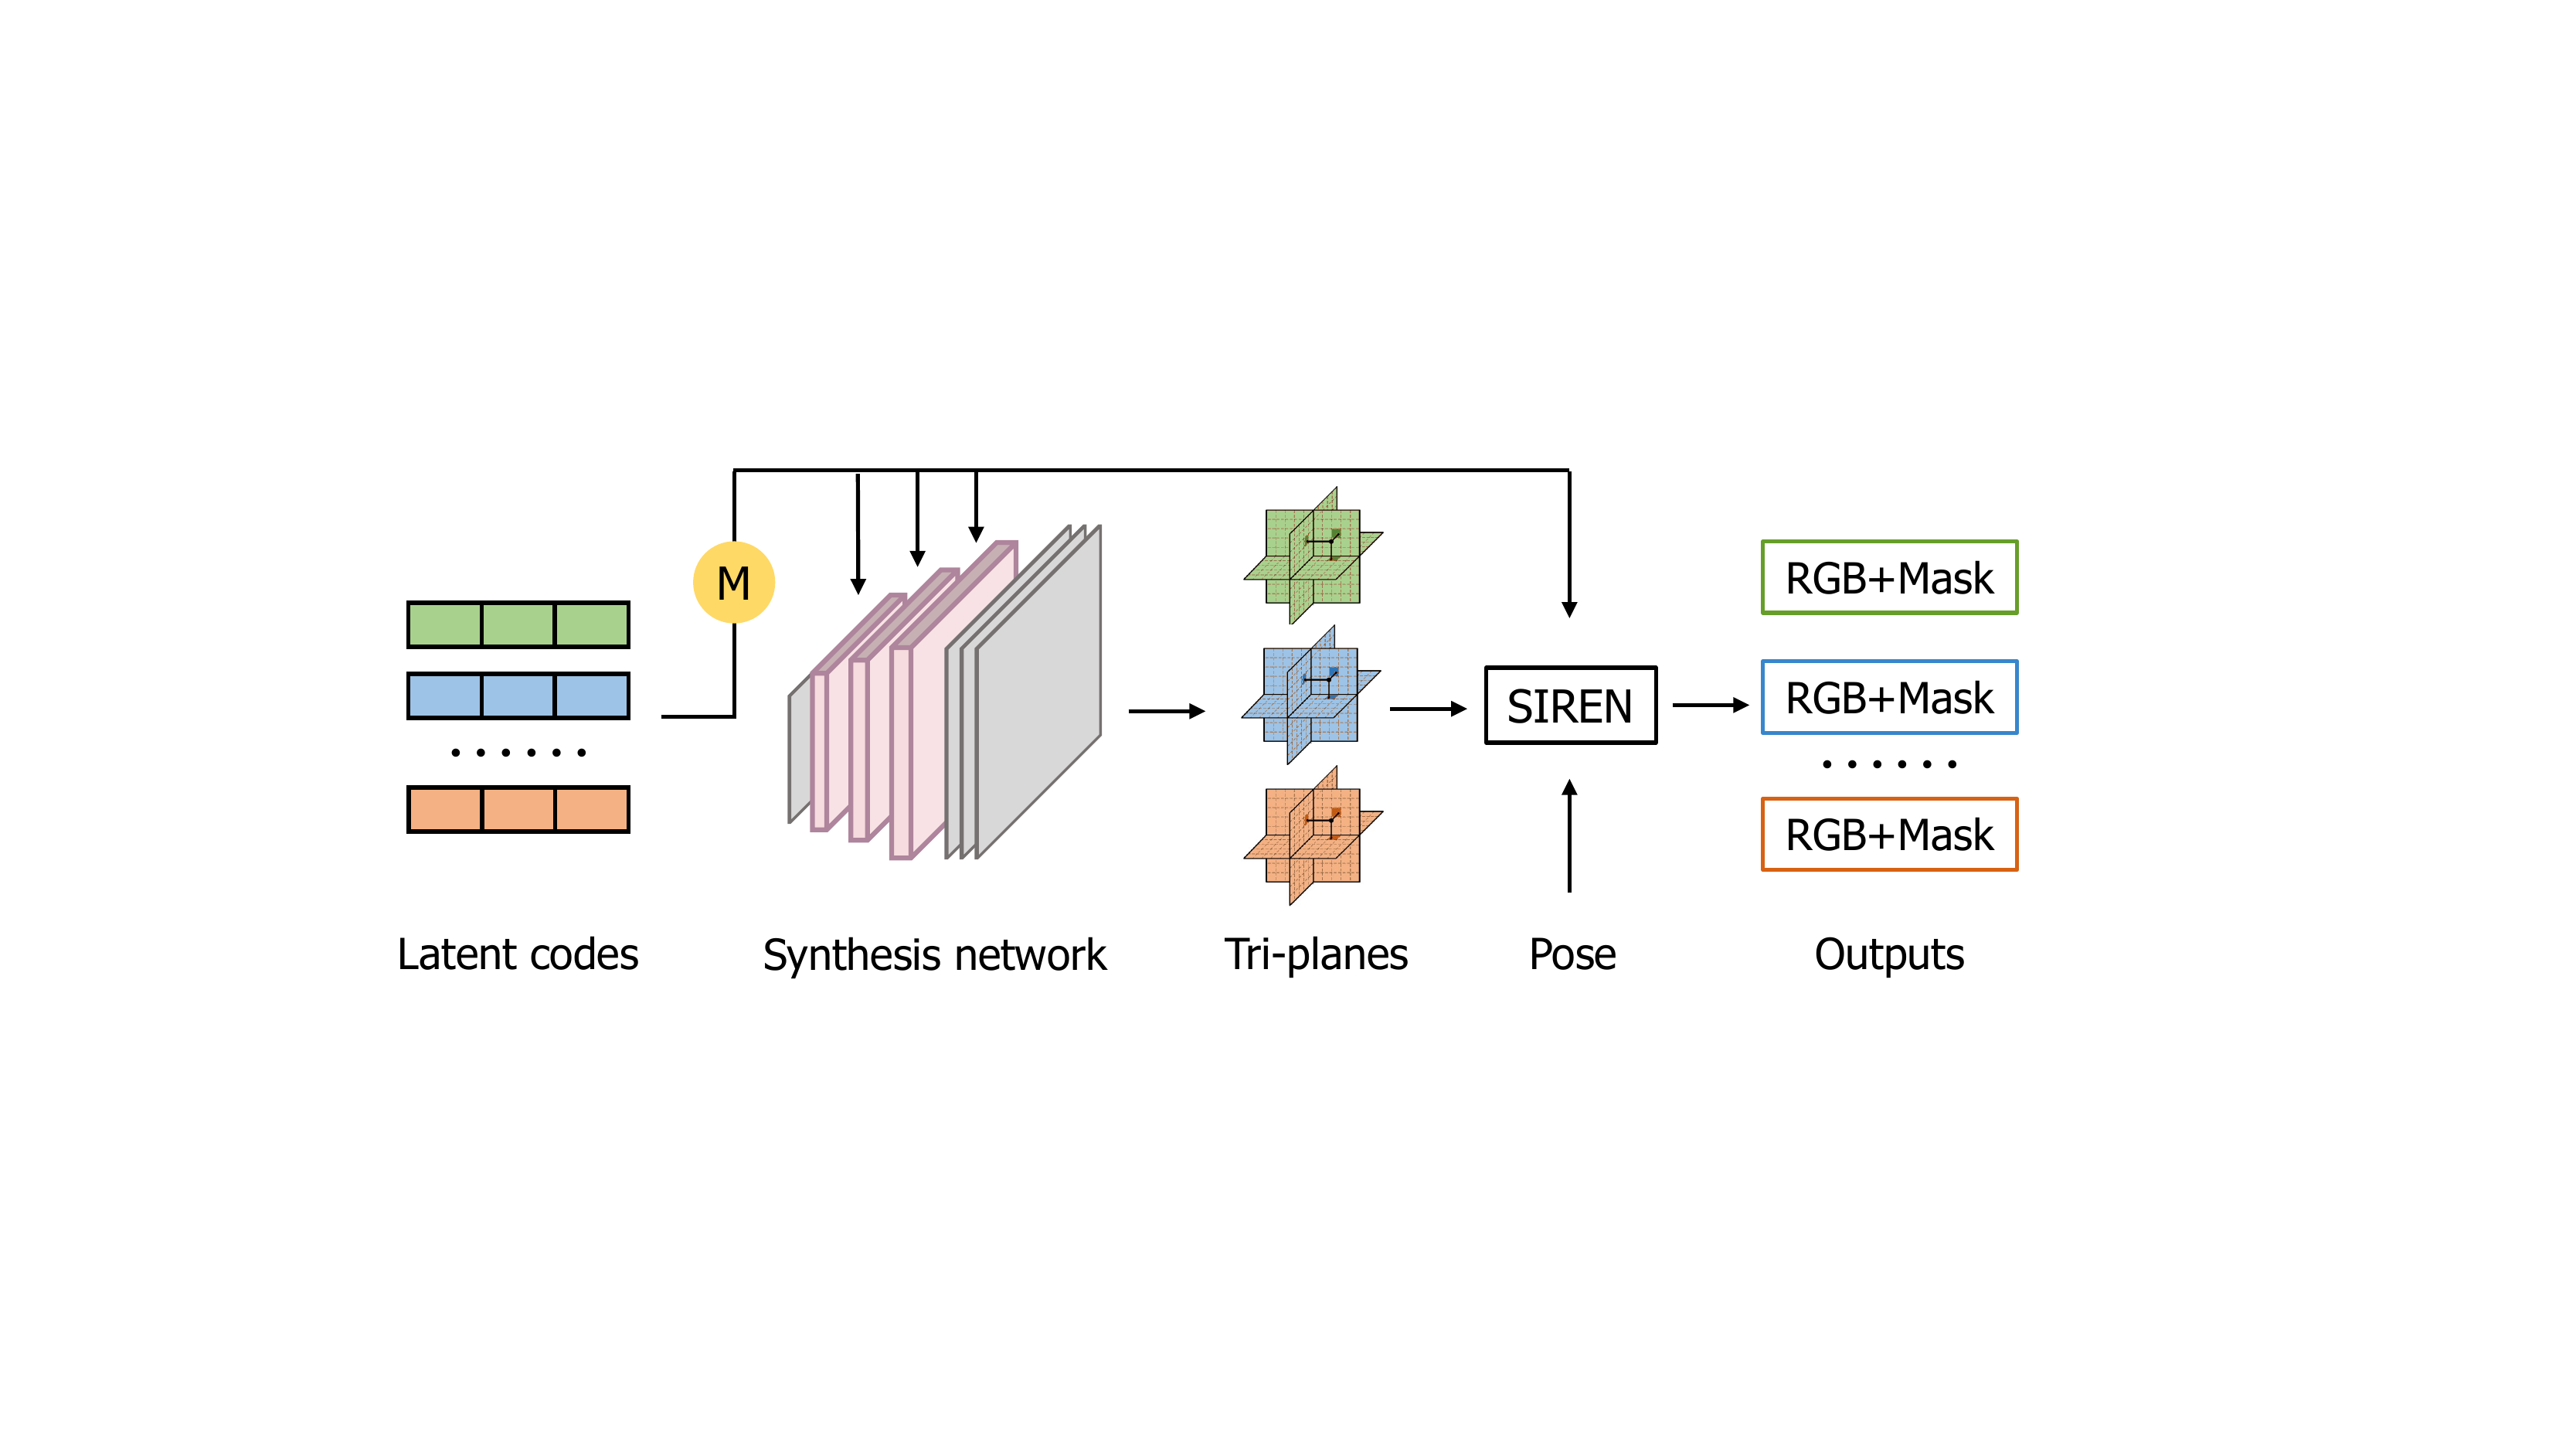}
    \caption{Network structure of NeRF in \textbf{Lift3D}, which converts latent codes to images and masks. $\mathbf{M}$ denotes the mapping network that maps latents $\mathbf{z}\in  \!\mathbb{R}^{512}$ to $\mathbf{w}\in  \!\mathbb{R}^{16\times 512}$. $\mathbf{w}$ are fed in AdaIN~\cite{huang2017arbitrary} to modulate the synthesis network to map the constant input to the tri-planes. SIREN is a single-layer MLP converts feature vector to RGB and density value.}
    \label{fig:nerf_supp}
\end{figure}

A normalized 3D bounding box~\cite{Wang_2019_CVPR} is utilized to filter out the background sampling points. During ray casting, we utilize an AABB-ray intersection algorithm~\cite{majercik2018ray} to find the nearest and furthest hitting points of 3D bounding box. The same parametrization can also be found in~\cite{Ost_2021_neuralscene,muller2022autorf}. The normalized sampling points lied in $[-1, 1]$ are projected to exactly cover the content of the tri-plane for tight parametrization. 

We further compare the lifting results of our shared NeRF with isolated NeRF in Fig.~\ref{fig:supp_compare}. Given the images generated from  StyleGAN2, we ablate two lifting processes: isolating training and joint training. The isolated NeRF is trained by optimizing the randomly sampled tri-planes and a single-layer SIREN to fit multi-view images. The shared NeRF is our proposed lifting process. We jointly optimize mapping network, synthesis network, SIREN, and a set of latents in the same time. The learned mapping network successfully maps randomly sampled latents $\mathbf{z}$ to object prior latent space $\mathbf{w}$ that can decoded by synthesis network to output meaning shape and appearance.

%  The learned mapping network expresses the underlying inductive bias that maps latents to gather in a tight latent space of a certain object category. 
 
% The same parametrization can also be found in~\cite{Ost_2021_neuralscene,muller2022autorf}. 

\section{Sample Parametrization}\label{sec:sam_p}

The final sampling pose $\mathbf{P}^{\prime}$ can be written as $(x,y,z,l,w,h,\theta )$, where $x, y, z$ is position of 3D bounding box, $l, w, h$ represent length, width, height of bounding box, $\theta$ is rotation along $y$ axis. We detail the parametrization of $\mathbf{P}^{\prime}$ in Tab.~\ref{tab:sam_p}.

% We uniformly sample position in $[-20m, 20m]$ for $x$ axis, $[5m, 45m]$ for $y$ axis. Object position for the $z$ axis is sampled from a Gaussian distribution that is centered at camera height. The rotation of object is considered as a bimodal distribution that is centered at forward facing($\pi / 2$) and backward facing($-\pi / 2$). Object sizes $l, w, h$ are also sampled from Gaussian distributions centered at mean size computed from each dataset.

\begin{table}[h!]
    \centering
    % \resizebox{0.7\linewidth}{!}{
    {
    \addtolength{\tabcolsep}{1pt}
    \centering

    \begin{tabular}{|l|c|c|c|c|c|c|}
    \hline
    {Pose} & {Distribution} &  {Parameters}   \\
    \hline
    $x$ & Uniform  & $[-20m, 20m]$  \\
    $y$ & Gaussian  & $\mu = height, \sigma = 0.2$  \\
    $z$ & Uniform  & $[5m, 45m]$  \\
    $l$ & Gaussian  & $\mu = l_{mean}, \sigma = 0.5$  \\
    $w$ & Gaussian  & $\mu = w_{mean}, \sigma = 0.5$  \\
    $h$ & Gaussian  & $\mu = h_{mean}, \sigma = 0.5$  \\
    $\theta$ & Gaussian  & $\mu = \pm \pi / 2, \sigma = \pi / 2$  \\

    \hline
    \end{tabular}%
    }

    \vspace{0.5mm}
    \caption{Detailed sampling parameters during composition. $l_{mean}$, $w_{mean}$ and $h_{mean}$ is the mean value of length, width, height of 3D box obtained from the statistic of datasets.}
    \label{tab:sam_p}
    % \vspace{-8mm}
\end{table}

\section{Multi-view Consistency}\label{sec:mvc}

% \myparagraph{Multi-view consistency}
% \quad 
We additionally compare multi-view consistency of our 3D generation framework with 3D generative model composed of a 2D upsampler. We use Reprojection Error (RE) proposed in~\cite{shi2022improving} to evaluate the consistency of generated images. We randomly choose two adjacent views, then render the images and corresponding depth map of the same object. We use the predicted depth to warp the image from one view to the other. The error is calculated between the predicted image and the warped image on 10K pairs.

\begin{table}[h!]

% \begin{wraptable}{r}{4.4cm}
    \centering

    \begin{tabular}{|l|c|c|c|c|c|c|}
    \hline
    \textbf{Method} &  {Reprojection Error}  \\
    \hline
    GIRAFFE~\cite{Niemeyer2020GIRAFFE} & 0.225 \\
    GIRAFFE HD~\cite{xue2022giraffehd} & 0.207 \\
    Ours & \textbf{0.079} \\
    \hline
    \end{tabular}%
    
    \caption{Comparison of multi-view consistency measured by Reprojection Error.
    }
    \label{tab:reproj_error}
    % \vspace{-8mm}
% \end{wraptable}
\end{table}

\begin{figure}[t!]
    \centering
    \includegraphics[width = 0.48\textwidth, trim = 0 0 0 0, clip]{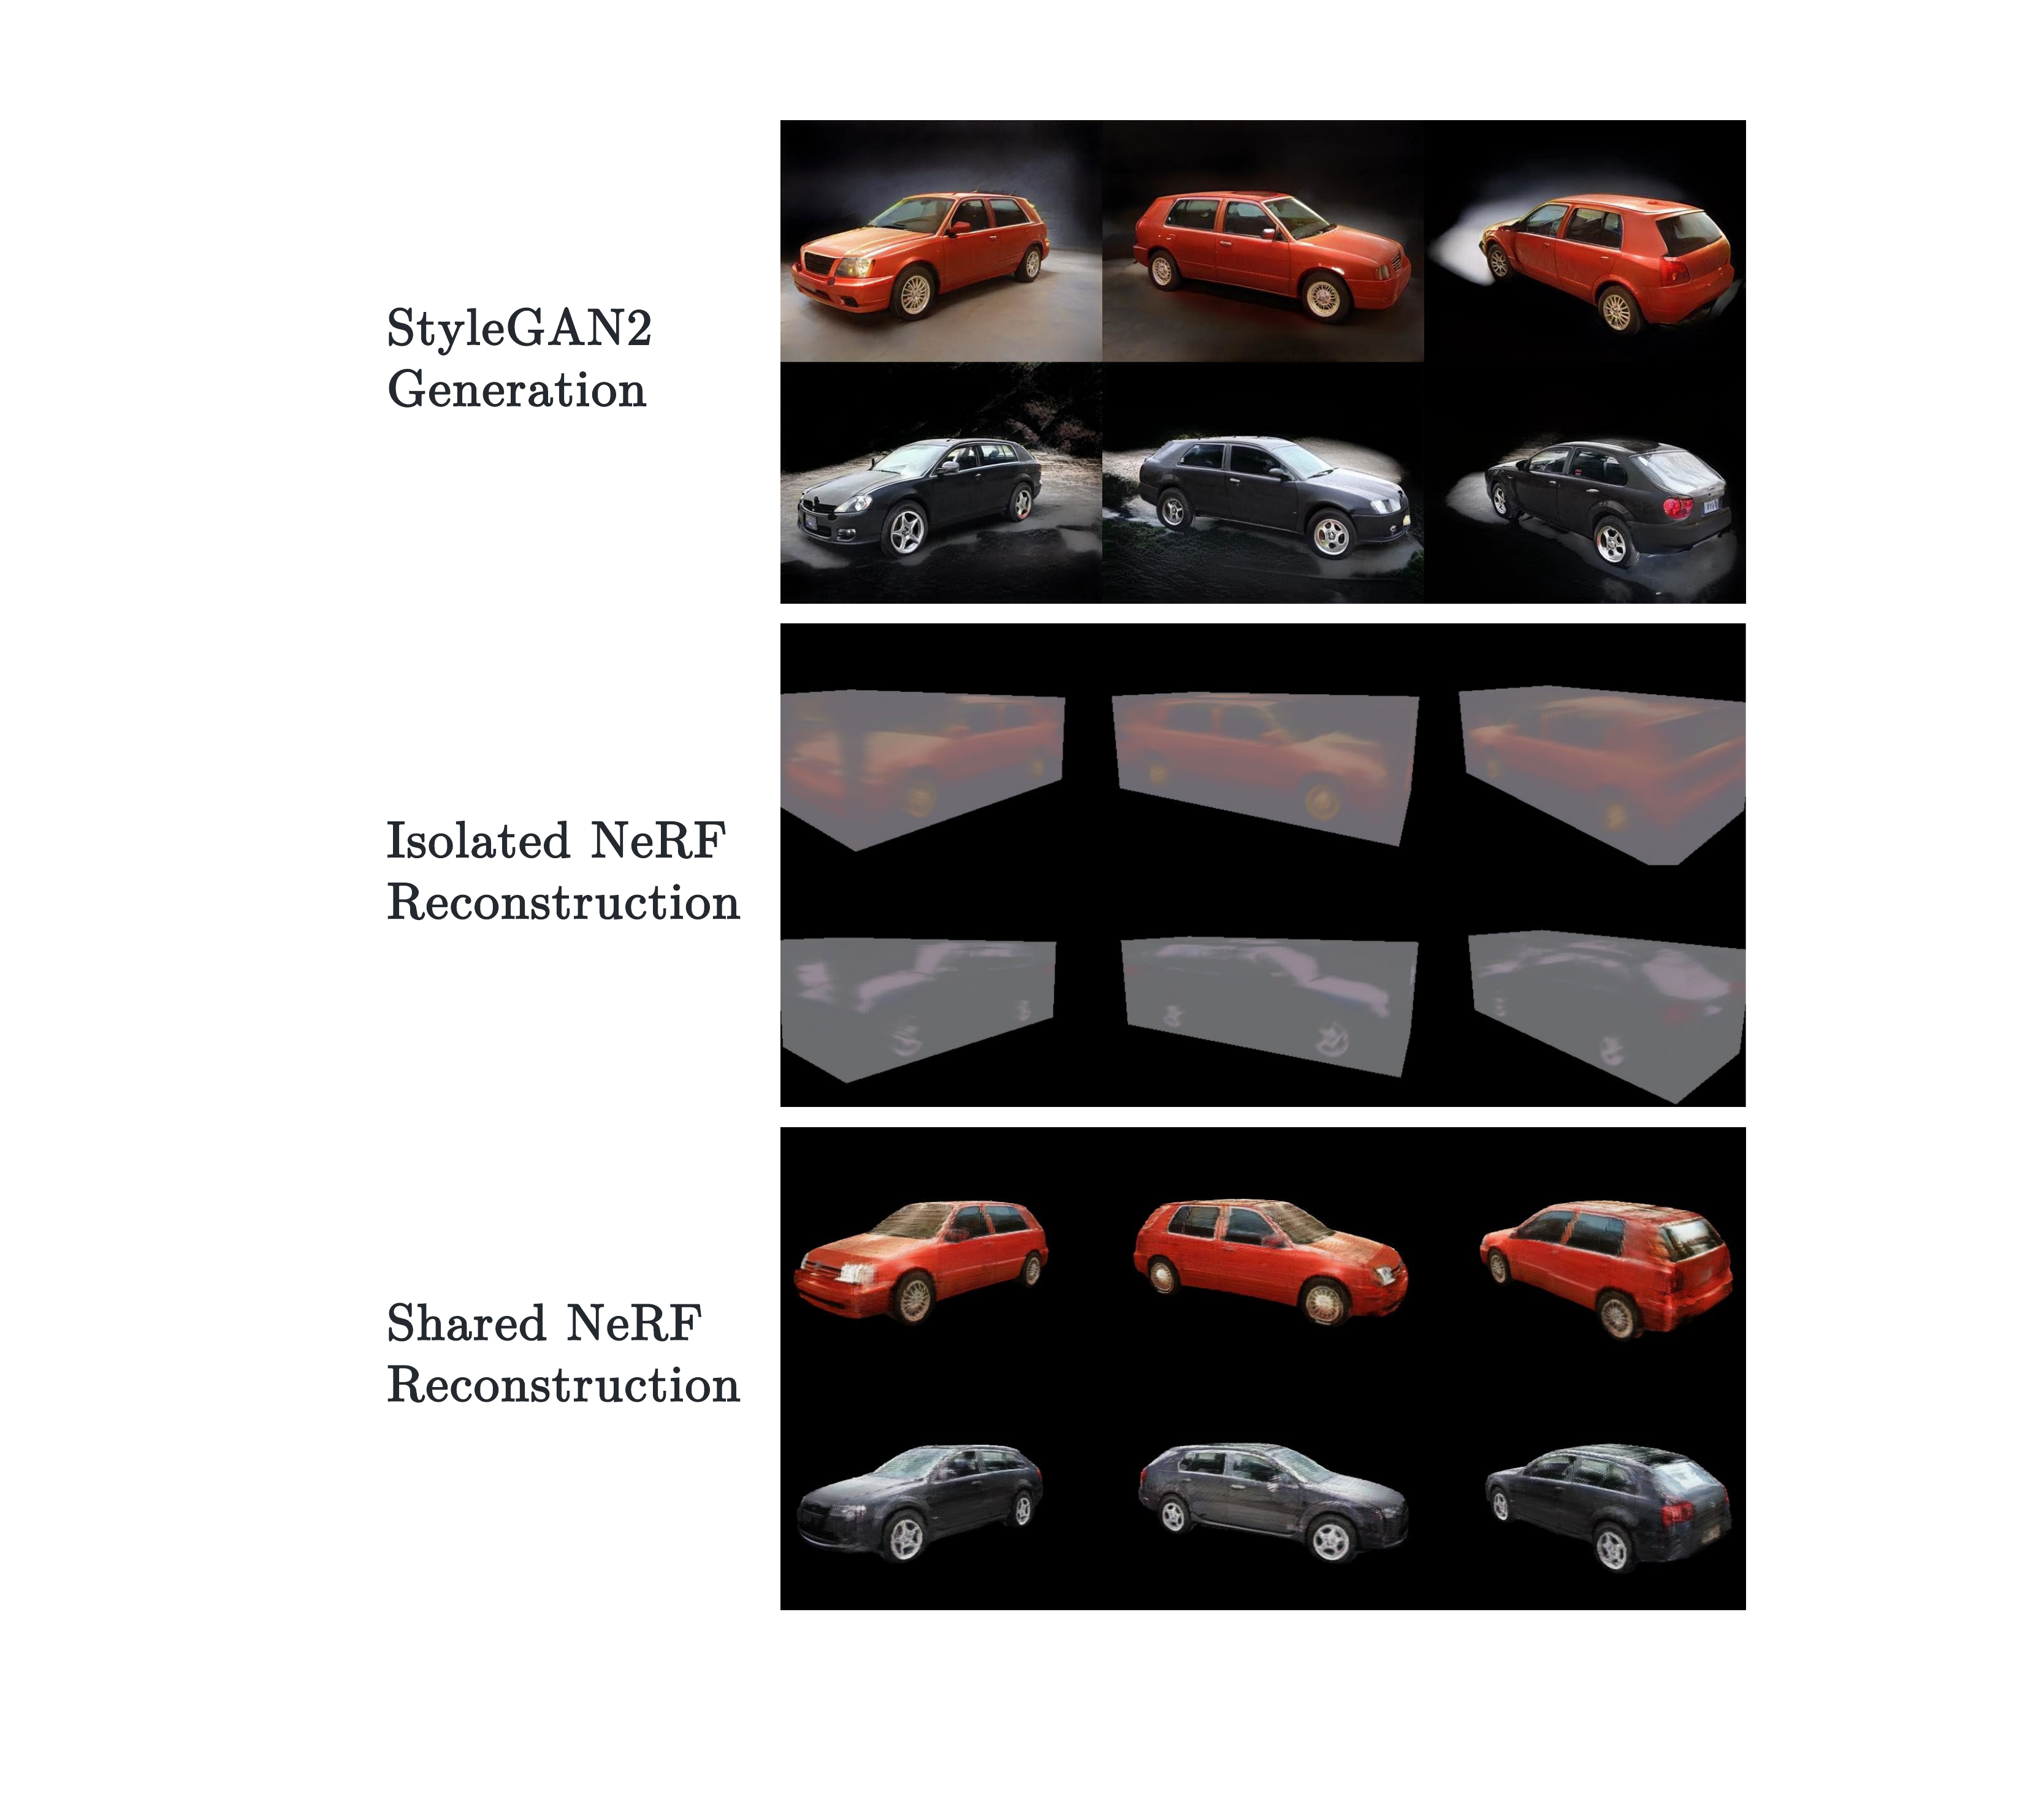}
    \caption{Qualitative comparison of our lifting process. Compared with training a large number of individual NeRFs, our method learns the object prior in the mapping network and synthesis network, which allows to use a single-layer MLP to generate diverse object radiance field.}
    \label{fig:supp_compare}
\end{figure}

\begin{figure*}[!htb]
    \centering
    \includegraphics[width = 0.9\textwidth, trim = 0 0 0 0, clip]{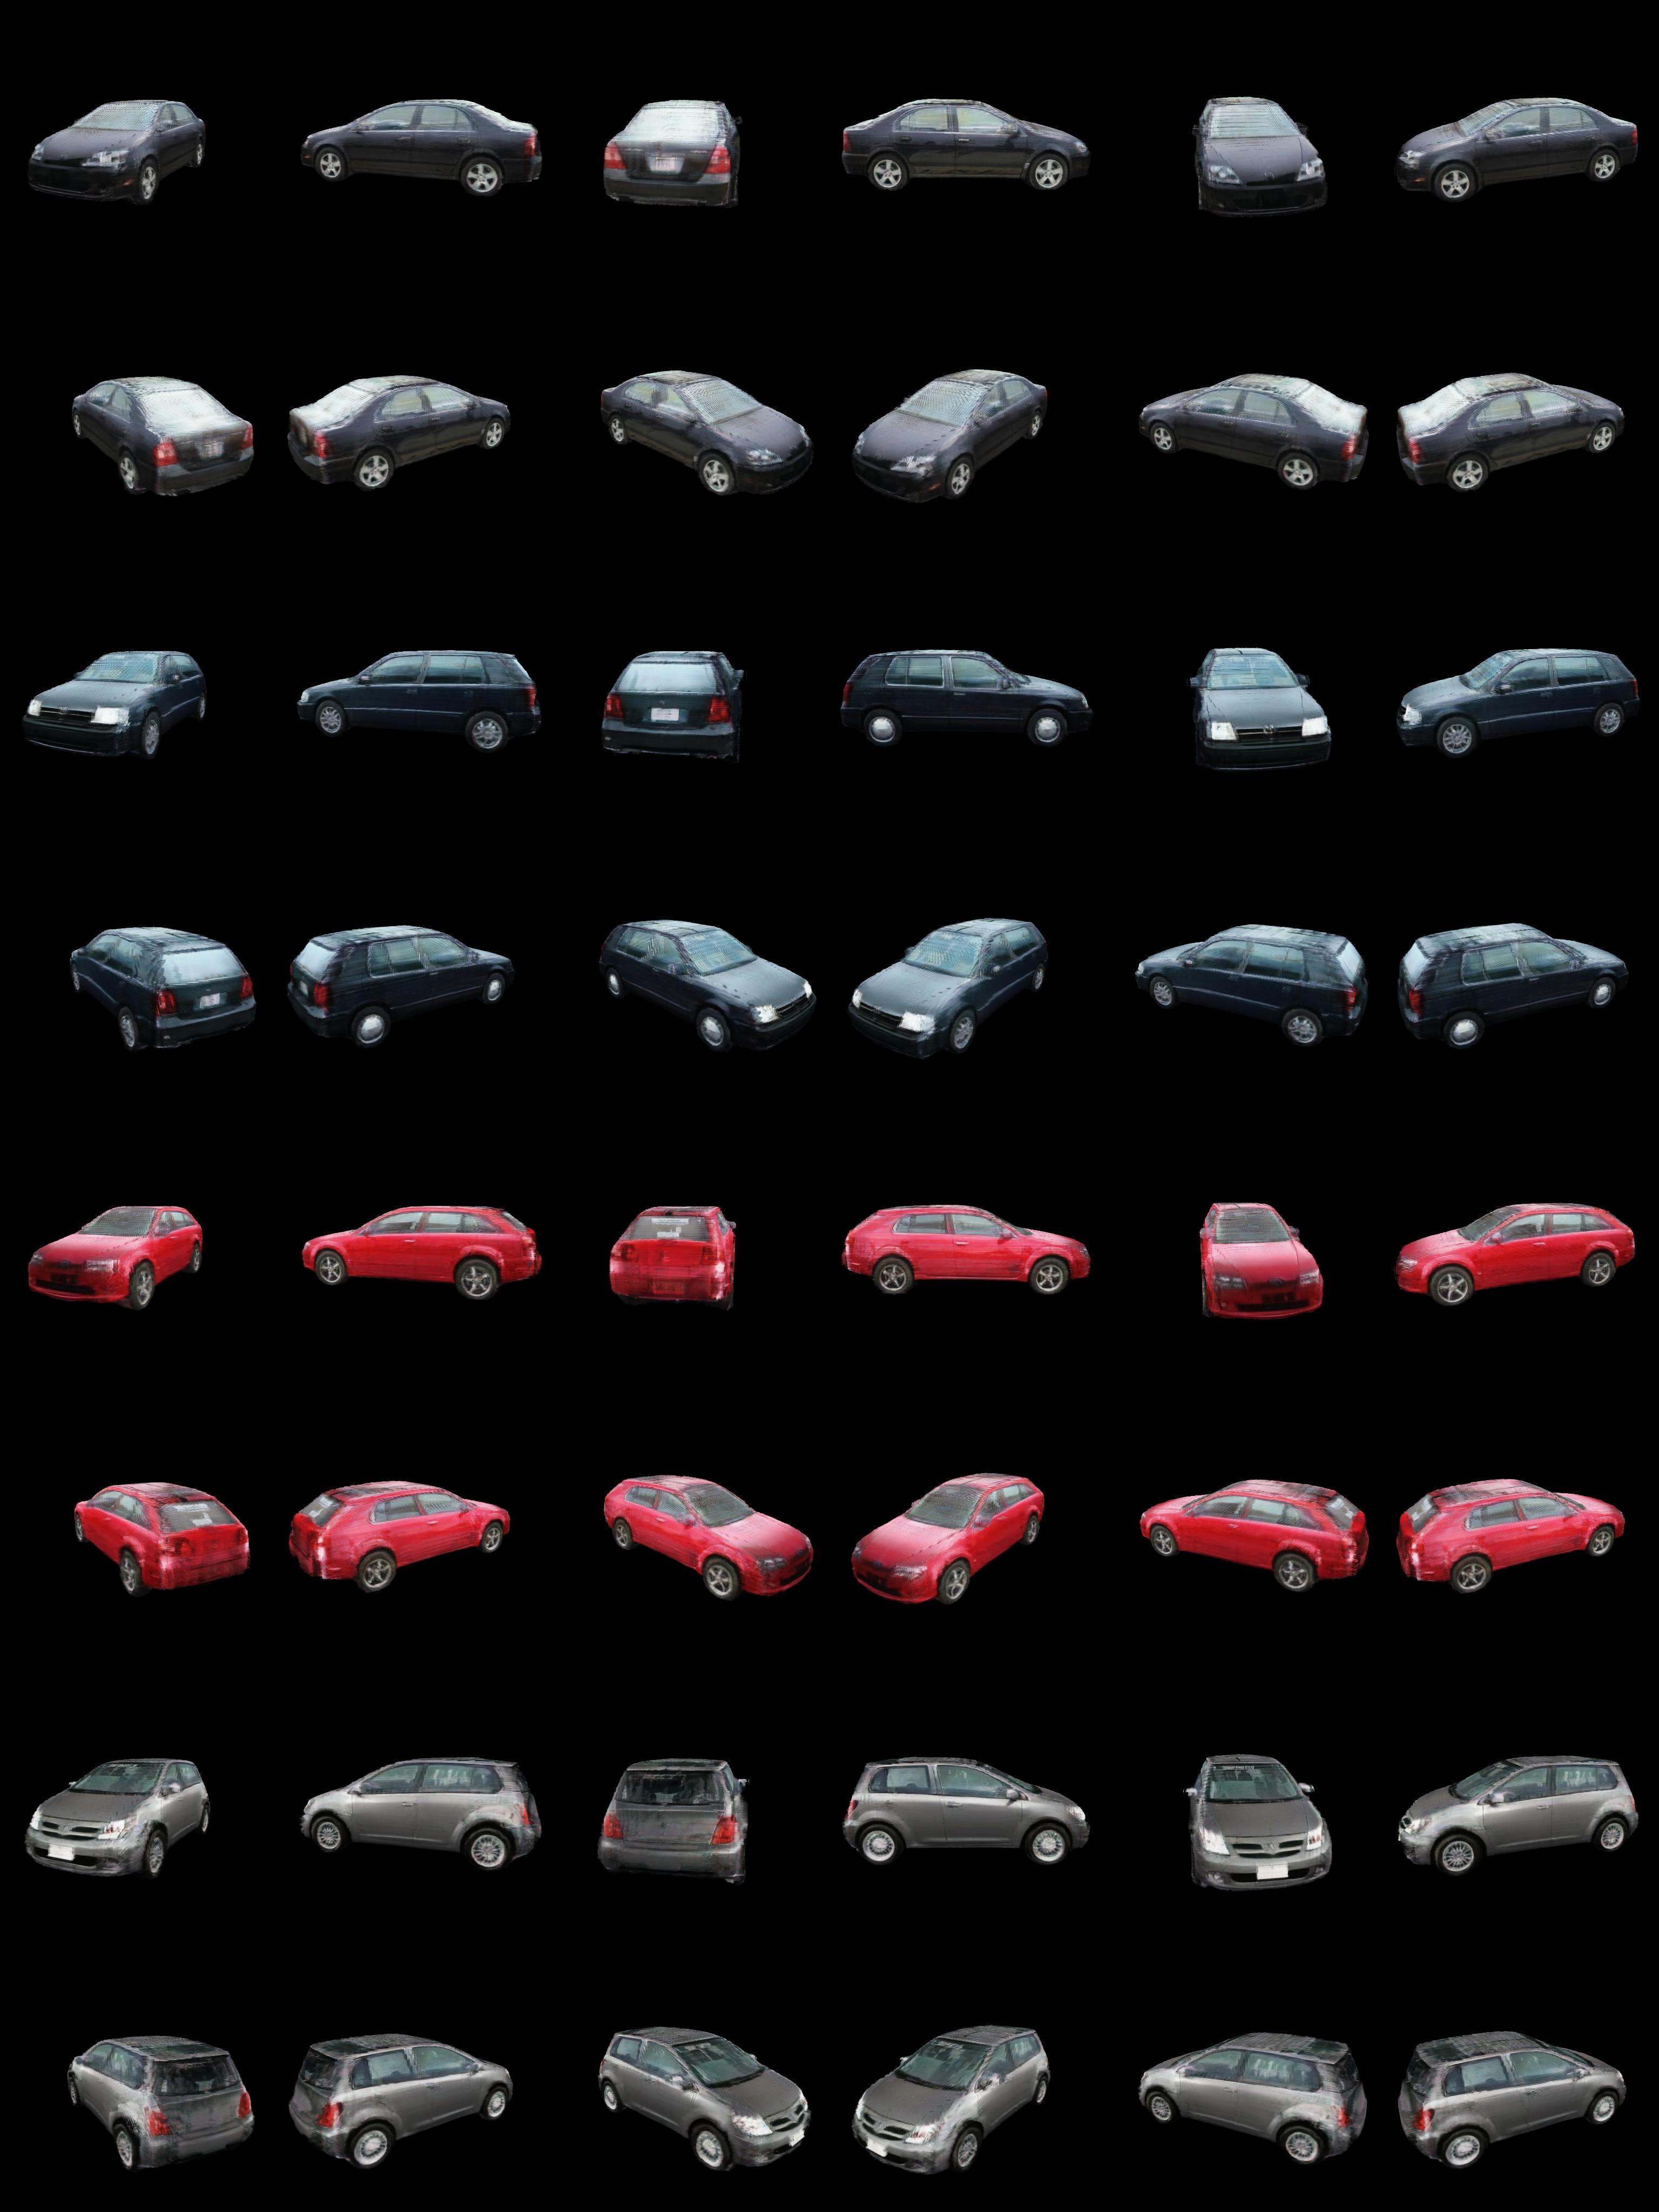}
    \caption{Novel view synthesis result of our generated objects.}
    \label{fig:mtv_4}
\end{figure*}
